# Supplementary material for: Step-Video-T2V Technical Report: The Practice, Challenges, and Future of Video Foundation Model
Source: arXiv:2502.10248 source file (2025-02-24)
Supplement: Supplementary file 2 [file a1_token_analysis.tex]

\section{Analysis and Visualization of Tokens in Pretraining}

\begin{figure*}[t]
\centering
\includegraphics[width=\textwidth]{figure/token_type_loss_7b.pdf}
\caption{\textbf{The loss of four categories of tokens during Mistral-7B pretraining on OpenWebMath.} (a) shows the loss of H→H, L→H, H→L, and L→L tokens during pretraining. (b) and (c) show three cases of fluctuating tokens' loss in L→L and H→H during pretraining, respectively.}
\label{fig:tokenppl_7b}
\end{figure*}

\subsection{More Details of Four Categories Tokens}
\label{sec:appendix:categorie_detail}

% \begin{figure*}[t]
% \centering
% \includegraphics[width=\textwidth]{figure/hhll_case.pdf}
% \caption{\textbf{Sample text containing four categories of tokens.} Among them, \textcolor[RGB]{30,144,255}{blue} represents tokens of categorie H→L, \textcolor[RGB]{34,139,34}{green} indicates tokens of categorie L→L, \textcolor[RGB]{250,170,0}{yellow} signifies tokens of categorie H→H, and \textcolor[RGB]{250,128,114}{red} denotes tokens of categorie L→H.}
% \label{fig:hhll_case}
% \end{figure*}

We categorize tokens into four categories: H→H, L→H, H→L, L→L. During the training process, we collected the loss of each token after training on each 1 billion tokens training data. We then used linear fitting and took the difference in loss between the first and last points as evidence of whether the loss decreased during the training process.

Specifically, suppose we have a sequence of token's loss $(l_0, l_1, ..., l_n)$. Our goal is to minimize the sum of the squares of the differences between each data point and its linear predictive value:

\begin{equation}
f(a, b) = \text{minimize} \sum_{i=0}^n (l_i - (ax_i + b))^2,
\label{equ:lossfitting}
\end{equation}

where $x_0=0$ is the initial checkpoint and $x_n=n$ is the final checkpoint. Substituting these into the fitted equation, we can obtain the Loss values at the start and end after fitting: $ \mathcal{L}_{\text{start}} = b$ and $\mathcal{L}_{\text{end}} = an + b$. The change in loss can then be expressed as: $\Delta \mathcal{L} = \mathcal{L}_{\text{end}} - \mathcal{L}_{\text{start}}$. Meanwhile, we represent the average Loss of the last checkpoint as $\mathcal{L}_{\text{mean}}$.

Next, we can classify the tokens based on $\Delta \mathcal{L}$ and the $\mathcal{L}_{\text{mean}}$. We categorize tokens with $\Delta \mathcal{L} < -0.2$ as H→L (loss decreases from high to low) category tokens, and tokens with $\Delta \mathcal{L} > 0.2$ as L→H (loss increases from low to high) category tokens. If $-0.2 \leq \Delta \mathcal{L} \leq 0.2$ and $l_n \leq \mathcal{L}_{\text{mean}}$, then tokens are classified as L→L (loss remains low); if $l_n >\mathcal{L}_{\text{mean}}$, they are classified as H→H (loss remains high). 
In \autoref{fig:tokenppl_7b}, we have added the tokens' loss curves of the 7B model which is consistent with the other experimental settings in \autoref{sec:analysis:dynamics}, for readers to refer to whether similar phenomena exist on larger models. 
In \autoref{fig:hhll_case}, we visualize examples of the four categories of tokens in actual text.

\subsection{Non-Converging Tokens in Pretrainig}
\label{sec:appendix:non_converging_token}
% orStagnant
% \begin{figure*}[t]
% \centering
% \includegraphics[width=\textwidth]{figure/token_fluctuating_example.pdf}
% \caption{\textbf{An example of an abnormal state of token perplexity during pretrainig process.} The tokens highlighted in \textcolor[RGB]{255,140,0}{orange} represent tokens that were significant abnormalities during the pretraining process.}
% \label{fig:token_fluctuating_example}
% \end{figure*}

In \autoref{sec:analysis:dynamics}, we mentioned that during the training process, only a minority of tokens belong to the H→L category. Among the remaining categories of H→H and L→L tokens, there are tokens that exhibit significant fluctuations during training. Furthermore, there are instances where H→L tokens are not effectively learned. Therefore, in our analysis, we specifically select those tokens from these categories that demonstrate considerable variability and distinct loss.
We visualize these tokens that exhibit abnormal behavior during the training process. As illustrated in \autoref{fig:token_fluctuating_example}, we find that the majority of these tokens originate from rather chaotic corpora. For instance, the corpora may include a mix of custom symbols, unintelligible gibberish, and information such as timetables and bibliographic references. Within a segment of normal text, there may also be fluctuations in the usage of common conjunctions, word suffixes, and punctuation marks. The latter may not necessarily be disastrous for training; in fact, it could represent a normal occurrence. However, if we can effectively mitigate the losses caused by the former, it might lead to more stable and efficient model training.
