# Supplementary material for: Step-Video-T2V Technical Report: The Practice, Challenges, and Future of Video Foundation Model
Source: arXiv:2502.10248 source file (2025-02-24)
Supplement: Supplementary file 8 [file a7_example_case.tex]

%\newpage

\begin{figure}[t]
\centering
\includegraphics[width=\textwidth]{figure/hhll_case.pdf}
\caption{\textbf{Sample text containing four categories of tokens.} Among them, \textcolor[RGB]{30,144,255}{blue} represents tokens of categorie H→L, \textcolor[RGB]{34,139,34}{green} indicates tokens of categorie L→L, \textcolor[RGB]{250,170,0}{yellow} signifies tokens of categorie H→H, and \textcolor[RGB]{250,128,114}{red} denotes tokens of categorie L→H.}
\label{fig:hhll_case}
\end{figure}

\begin{figure}[t]
\centering
\includegraphics[width=\textwidth]{figure/token_fluctuating_example.pdf}
\caption{\textbf{An example of an abnormal state of token perplexity during pretrainig process.} The tokens highlighted in \textcolor[RGB]{255,140,0}{orange} represent tokens that were significant abnormalities during the pretraining process.}
\label{fig:token_fluctuating_example}
\end{figure}

\begin{figure}[t]
\centering
\includegraphics[width=\textwidth]{figure/token_select_example.pdf}
\caption{\textbf{Specific examples of selecting tokens during the selective pretraining process of the \model{}.} The tokens marked in \textcolor[RGB]{30,144,255}{blue} represent the actual tokens trained during the training process, while the remaining black tokens are not trained during the training process.}
\label{fig:token_select_example}
\end{figure}

\begin{figure}[t]
\centering
\includegraphics[width=\textwidth]{figure/example_dynamic_token.pdf}
\caption{\textbf{An example of dynamic token selection changes during the training process}, which illustrated with five different score levels represented by \textcolor[RGB]{0,0,255}{deep blue}, \textcolor[RGB]{30,144,255}{light blue}, black, \textcolor[RGB]{255,180,150}{light orange}, and \textcolor[RGB]{255,100,0}{dark orange}. The bluer the color indicates a higher tendency for the token to be selected, while the more orange the color suggests a lower tendency for the token to be selected.}
\label{fig:example_dynamic_token}
\end{figure}
